# Supplementary material for: Distribution Estimation for Probabilistic Loops
Source: arXiv:2205.07639 source file (2022-05-13)
Supplement: Supplementary file 1 [file Appendix1.tex]

\newpage

\section{Appendix A: Estimation of Known Distributions}

% \subsection{Cauchy Distribution}

% \todo{explain more!!!}

% The Cauchy distribution has the probability density function 
% \begin{align*}
%     f(x)=\frac{1}{\pi\gamma\Big[1+\Big(\frac{x-x_0}{\gamma}\Big)^2\Big]}
% \end{align*}
% where $x_0$   is the location parameter specifies location of the peak of the distribution, and  the scale parameter $\gamma$   specifies half the width of the PDF at half the maximum height.

% %%%%%%%%%%%%%%%%%%%%%%%%%%%%%%%%%%%%%%%%%%%%%%%%%%%%
% \begin{figure}[tpbh!]
% 	\centering
% 	\includegraphics[width=4.2cm]{Figures/MEforCauchyDist6moments.eps}
% 	\caption{Maximum Entropy with 6 moments: Standard Cauchy Distribution.}
% 	\label{fig:MEforChauchyDist6moments}
% \end{figure}

% %%%%%%%%%%%%%%%%%%%%%%%%%%%%%%%%%%%%%%%%%%%%%%%%%%%%
% %%%%%%%%%%%%%%%%%%%%%%%%%%%%%%%%%%%%%%%%%%%%%%%%%%%%
% \begin{figure}[tpbh!]
% 	\centering
% 	\includegraphics[width=4.2cm]{Figures/GramCharlierCauchyDist4Cumulants.eps}
% 	\includegraphics[width=4.2cm]{Figures/GramCharlierCauchyDist8Cumulants.eps}
% 	\caption{Gram-Charlier for Standard Cauchy Distribution: with 4 cumulants (left), with 8 cumulants (right)}
% 	\label{fig:GramCharlierforChauchyDist6moments}
% \end{figure}

% \bigskip
% %\newpage
\subsection{Normal Mixture Distribution}

%\addnote{explain more!!!}

Normal mixture: $f(x)=\alpha N(\mu_1,\sigma_1)+(1-\alpha) N(\mu_2,\sigma_2)$, $\alpha \in (0,1)$.
\begin{figure}[tpbh!]
	\centering
	\includegraphics[width=3.8cm]{Figures/MEforNormalMixture.eps}
	\includegraphics[width=3.8cm]{Figures/MEforNormalMixturealph05.eps}
	\includegraphics[width=3.8cm]{Figures/MEforNormalMixturealpha018.eps}
	\caption{Maximum Entropy for Normal Mixture with $\mu_1=-2, \sigma_1=1, \mu_2=1, \sigma_2=1$:   $\alpha=0.85$ (left),  $\alpha=0.5$ (middle), $\alpha=0.19$ (right).}
	\label{fig:MEforNormalMixtureDist6moments}
\end{figure}

\begin{figure}[tpbh!]
	\centering
	\includegraphics[width=3.8cm]{Figures/GramCharlierforNormalMixture4cumulantsalpha085.eps}
	\includegraphics[width=3.8cm]{Figures/GramCharlierforNormalMixture4cumulantsalpha05.eps}
	\includegraphics[width=3.8cm]{Figures/GramCharlierforNormalMixture4cumulantsalpha019.eps}\\
	\includegraphics[width=3.8cm]{Figures/GramCharlierforNormalMixture8cumulantsalpha0850.eps}
	\includegraphics[width=3.8cm]{Figures/GramCharlierforNormalMixture8cumulantsalpha05.eps}
	\includegraphics[width=3.8cm]{Figures/GramCharlierforNormalMixture8cumulantsalpha019.eps}
	\caption{Maximum Entropy for Normal Mixture with $\mu_1=-2, \sigma_1=1, \mu_2=1, \sigma_2=1$: (top: 4 cumulants, bottom: 8 cumulants);  $\alpha=0.85$ (left),  $\alpha=0.5$ (middle), $\alpha=0.19$ (right).}
	\label{fig:GramCharlierforNormalMixtureDist}
\end{figure}

%%%%%%%%%%%%%%%%%%%%%%%%%%%%%%%%%%%%%%%%%%%%%%%%%%%%
% \bigskip
% \newpage
% \subsection{Gamma Distribution}

% \subsection{Gompertz Distribution}
% .
% \bigskip
\subsection{Weibull Distribution}

%\addnote{explain more!!!}

The PDF of Weibull random variable is 
\begin{align*}
    f(x;\lambda,k)=\Big\{
    \begin{matrix}
         \frac{k}{\lambda}(\frac{x}{\lambda})^{k-1}e^{-(x/\lambda)^k}& & x\geq 0, \\
          0& &  x<0,\\
    \end{matrix}
\end{align*}
where $k>0$ is the shape parameter and $\lambda>0$ is the scale parameter of the distribution.
\begin{figure}[tpbh!]
	\centering
	\includegraphics[width=4.2cm]{Figures/MEforWeibull.eps}
		\caption{Maximum Entropy for Weibull Distribution  with $k=1.5, \lambda=1$.}
	\label{fig:MEforWeibull6moments}
\end{figure}

\begin{figure}[tpbh!]
	\centering
	\includegraphics[width=4.2cm]{Figures/GramCharlierforWeibull4cumulants05.eps}
	\includegraphics[width=4.2cm]{Figures/GramCharlierforWeibull8cumulants05.eps}
	\caption{Gram-Charlier for Weibull Distribution  with $k=1.5, \lambda=1$:   4 cumulants (left),  8 cumulants (right).}
	\label{fig:GramCharlierforWeibull}
\end{figure}

% \subsection{Hotelling's T-squared Distribution}

% \subsection{Truncated Normal Distribution}

% \subsection{Half-normal Distribution}

% \subsection{F-distribution}

% \subsection{Generalized Extreme Value Distribution}

% \subsection{Gumbel Distribution}
%\newpage

\subsection{Numerical Results}
% \begin{itemize}
% \item The {\bf Hellinger Distance} is used to quantify the similarity between two probability distributions.  Let $p(x)$ and $q(x)$ are pdfs of true and estimated distributions, respectively.  The square of the Hellinger distance is defined as follows: 
% \begin{align*}
%     H^2(P,Q)&=\frac{1}{2}\int\Big(\sqrt{p(x)} - \sqrt{q(x)}\Big)^2dx \\
%     &= 1-\int\sqrt{p(x)q(x)} dx.
% \end{align*}
% Note that $0\leq H(P,Q) \leq 1$.

% \item 
{\bf Kullback–Leibler Divergence},  $D_{\text{KL}}$ quantifies how much one probability distribution differs from another probability distribution.
To measure the difference between two probability distributions over the same
variable $X$,  the Kullback-Leibler divergence, or simply, the KL
divergence, has been popularly used in the data mining literature and it is a non-symmetric measure of the difference between two probability distributions $p(x)$ and $q(x)$. Here we assume that $p(x)$ is the true (known) distribution and $q(x)$ is an approximation of $p(x)$.  The continuous version of KL divergence is 
\begin{align}
    D_{KL}(P||Q) = \int_{-\infty}^{\infty} p(x)\ln\frac{p(x)}{q(x)}dx.
\end{align}
$D_{KL}(P||Q)$ is non-negative  and $D_{KL}(P||Q)=0$ if and only if $P = Q$.

%\end{itemize}

\bigskip
\begin{table}[tpbh!]
    \centering
 \begin{tabular}{|c|c|c|c|}
\hline
              & ME& GC &GC\\
              & (6 mom.)& (4 cumul.)&(8 cumul.)\\
              \hline
    %  Example 1& 0.0328& 0.1002 &0.0148\\\hline
    %  Example 2& 0.0139&0.1373 & 0.0360\\\hline
     Cauchy & 0.8516& 0.3684& 0.2990\\\hline
     Normal Mixture& 0.0236 & 0.0399 &0.0012\\\hline
     Weibull& 0.0105 & 0.0614 & 0.0407\\\hline
     
\end{tabular}
 \caption{Kullback-Leibler divergence ($D_{KL}$ of true and estimated  distributions with Maximum Entropy (ME) and Gram-Charlier (GC)).}
     \label{table:Kullback-LeiblerDivergence} 
        
\end{table}

%\todo{to do /////}

\bigskip
\bigskip
