# Supplementary material for: Distribution Estimation for Probabilistic Loops
Source: arXiv:2205.07639 source file (2022-05-13)
Supplement: Supplementary file 2 [file Appendix2.tex]

\section{Appendix B: Second Moment of StutteringP}

%\addnote{Type the calculation!}

With a closer look at the StutteringP probabilistic program in Table~\ref{table:BenchmarkPrograms} we can see that \begin{align}
    & E[f(n+1)]= p E[1] + (1-p) E[0],\\
    & E[x(n+1)]= E[x(n)+ f(n+1)\cdot rand(0,2)],\label{eq:firstmomentStutteringPCalculations-1}\\
    & E[y(n+1)]= E[y(n)+ f(n+1)\cdot rand(0,4)],\label{eq:firstmomentStutteringPCalculations-2}\\
    &  E[s(n+1)]= E[x(n+1)+ y(n+1)].
\end{align}
which leads to 
\begin{align}
    & E[f(n+1)]= p,\\
    & E[x(n+1)]= E[x(n)]+ E[f(n+1)]\cdot E[rand(0,2)],\\
    & E[y(n+1)]= E[y(n)]+ E[f(n+1)]\cdot E[rand(0,4)],\\
    &  E[s(n+1)]= E[x(n+1)]+E[y(n+1)].
\end{align}
Then we can write the recurrence relations. Solving this recurrences leads us to the close form of first moments, i.e. expectation, of each involved variables. 
\begin{align}
    & E[f(n)]= p,\label{eq:firstmomentStutteringPCalculations1}\\
    & E[x(n+1)]= E[x(n)]+ p \;\Longrightarrow \; E[x(n)]=np-1 \; \text{ as } \; x(0)=-1,\label{eq:firstmomentStutteringPCalculations2}\\
    & E[y(n+1)]= E[y(n)]+ 2p \;\Longrightarrow \; E[y(n)]=2np+1 \; \text{ as } \; y(0)=1,\label{eq:firstmomentStutteringPCalculations3}\\
    &  E[s(n)]= E[x(n)]+E[y(n)]= np-1+2np+1 \;\Longrightarrow \; E[s(n)]=3np. 
\end{align}

Now we calculate recurrences and closed forms for the second moments of involved variables. As  $E[f(n+1)^2]=p E[1^2] + (1-p) E[0^2] = p$, we conclude that 
\begin{align}
    E[f(n)^2]=p.
\end{align}
For other variables
\begin{align}
   E[x(n+1)^2] & = E[\big(x(n)+ f(n+1)\cdot rand(0,2)\big)^2]\notag\\
             & = E[x(n)^2]+ 2E[x(n)] E[f(n+1)]E[rand(0,2)] \notag\\
             & \hspace{2.8cm}+ E[f(n+1)^2] E[rand(0,2)^2]\notag\\
             & = E[x(n)^2]+ 2E[x(n)] E[f(n+1)] + E[f(n+1)^2] \frac{4}{3}\notag\\
             & = E[x(n)^2]+ 2E[x(n)] E[f(n+1)] + E[f(n+1)^2] \frac{4}{3}
\end{align}
Considering Equations~\eqref{eq:firstmomentStutteringPCalculations1} and \eqref{eq:firstmomentStutteringPCalculations2} we have following recurrence for the second moment of random variable $x$:
\begin{align}
   E[x(n+1)^2] = E[x(n)^2]+ 2(np-1)p +  \frac{4}{3}p.
\end{align}
To solve this recurrence we have
\begin{align*}
   E[x(n)^2] &= E[x(0)^2]+ \sum_{i=0}^{n-1}\Big(2(ip-1)p +  \frac{4}{3}p\Big)\\
   & = E[x(0)^2]+ 2p^2\Big(\sum_{i=0}^{n-1} i\Big)+ n(-2p+\frac{4}{3}p)\\
   &=1+ 2p^2\Big(\frac{(n-1)(n)}{2}-\frac{2np}{3},
\end{align*}
which leads us to the closed form for second moment of $x$ in StutteringP:
\begin{align}
   E[x(n)^2] &= n^2p^2 - np^2 -\frac{2}{3}np+1.
\end{align}
The same calculations and considering Equations ~\eqref{eq:firstmomentStutteringPCalculations1} and \eqref{eq:firstmomentStutteringPCalculations3}, we reach 
\begin{align}
   E[y(n)^2] &= 4n^2p^2 - 4np^2 -\frac{28}{3}np+1.
\end{align}
To obtain recurrence relation for random variable $s$ we consider 
\begin{align*}
   E[s(n+1)^2]&=E[\Big(x(n+1)+y(n+1)\Big)^2]\\
              &= E[x(n+1)^2] + 2E[(xy)(n+1)]  + E[y(n+1)^2] 
\end{align*}
in which $E[(xy)(n+1)]$ can be represented as a recurrence by multiplication of recurrences of $E[x(n+1)]$ and $E[y(n+1)]$ in \eqref{eq:firstmomentStutteringPCalculations-1} and \ref{eq:firstmomentStutteringPCalculations-2}:
\begin{align*}
  E[(xy)(n+1)]&= E[(xy)(n)] + 2 E[x(n)] E[f(n+1)] + E[y(n)] E[f(n+1)]+ 2E[f(n+1)^2] \\
  &= E[(xy)(n)] + 2(np-1)p + (2np+1)p +2p
\end{align*}
Solving this recurrence we obtain
\begin{align*}
  E[(xy)(n)]&= E[(xy)(0)] + \sum_{i=0}^{n-1}\Big(2ip^2-2p+2ip^2+p+2p\Big)\\
  &=2n^2p^2 -2np^2+np-1.
\end{align*}
Finally we obtain a closed form  for the second moment of random variable $s$:
\begin{align*}
   E[s(n)^2]&=E[\big(x(n)+y(n)\big)^2]\\
              &= E[x(n)^2] + 2E[(xy)(n)]  + E[y(n)^2]\\
              &=(n^2p^2 - np^2 -\frac{2}{3}np+1)+2(2n^2p^2 -2np^2+np-1)+(4n^2p^2 - 4np^2 -\frac{28}{3}np+1)\\
              & = 9n^2p^2 - 9np^2+ 32np.
\end{align*}
