# Supplementary material for: Distribution Estimation for Probabilistic Loops
Source: arXiv:2205.07639 source file (2022-05-13)
Supplement: Supplementary file 3 [file Appendix.tex]

\section*{Appendix}\label{Appendix}

Table~\ref{table:BenchmarkPrograms} shows the description of selected prob-solvable probabilistic programs as benchmarks. For more, see \cite{bartocci2019automatic}. 
\vspace{-5mm}
\begin{table}[tpbh!]
    \centering
    \scalebox{0.6}{
 \begin{tabular}{clc|clc|clc|clc|clc}
\toprule
    %   \multirow{3}{*}{} 
    %   &&&&& &&&& && &&&\\
\hspace{1mm}&{\bf StutteringP}&\hspace{1mm}&\hspace{1mm}& {\bf Square} & \hspace{1mm}&\hspace{1mm}&  {\bf Binomial($p$)} \hspace{1mm} & \hspace{1mm}&\hspace{1mm}& {\bf Random Walk 1D } &  &\hspace{1mm} &{\bf Uniform}&\hspace{1mm} \\
%&&&&&&&&&&&&&&\\
\midrule
%&&&&&&&&&&&&&&\\
&$f:=0$&&& $x:=0$ &&& $x:=0$ && & $v:=0$& &&$x := 1/2$&\\
&$x:=-1$&&& $y:=1$ &&&$\text{while true:}$&& & $x:=0$& &&$u := 0$&\\
&$y:=1$&&& $\text{while true:}$ &&&$\quad x:=x+1\;\;[\;p\;]\;\;x$ &&  & $\text{while true:}$& && $\text{while true:}$ &\\
&$s:=0$&&& $\quad x:=x+2\;\;[0.5]\;\;x$  &&&&& &$\quad v:=\text{unif.}(0,1)$& &&$\quad u:=u\;\;[0.5]\;\;u+x$&\\
&$\text{while true:}$&&& $\quad y:=x^2$ &&&&& &$\quad x:=x+v\;\;[0.7]\;\;x-v$& && $\quad  x := x/2$ &\\
&$\quad f:=1\;\;[\;{ p }\;]\;\;0$&&&  &&&&& && &&&\\
&$\quad x:=x+f*\text{unif.}(0,2)$&&&  &&&&& && &&&\\
&$\quad y:=y+f*\text{unif.}(0,4)$&&&  &&&&& &&. &&&\\
&$\quad s:=x+y$&&&&  &&&& && &&&\\
%&&&&&  &&&& && &&&\\
                         \bottomrule

\end{tabular}
}
\vspace{2mm}
 \caption{Benchmark Programs.}
    \label{table:BenchmarkPrograms}
        
\end{table}

\appendix\label{appendixB}

\paragraph{\bf General Loops in Probabilistic Programs: }

We consider the  stochastic differential equation,
\begin{align}\label{eq:SDE2}
    dX(t)= -\frac{1}{4}X^3(t) dt -\frac{1}{2}X^2(t) dW(t) \quad \text{with} \quad X(0)=2,
\end{align}
where $W$ denotes the Wiener process (standard Brownian motion) \cite{morters2010brownian}. Eqn. \eqref{eq:SDE2} can be represented as the probabilistic program in the left panel of Figure~\ref{fig:HistogramPDFCDFofGeneralLoopEx1}.
\begin{figure}[tpbh!]
	\centering
	\begin{minipage}{0.42\textwidth}
	\begin{align*}
&x:=2, w:=0\\\notag
%&w:=0\\\notag
&dt:=1, \sigma:=0.1\\\notag
%&\sigma:=0.1\\\notag
&\text{\bf while } true \text{ \bf do}\\\notag
&\quad w:=\text{Normal}(0,1)\\\notag
&\quad x:=x-\frac{1}{4}x^3\ast dt -\frac{1}{2}x^2\ast \sigma\ast w\\
& \text{\bf end while }
\end{align*}
	\end{minipage}
	\begin{minipage}{0.56\textwidth}
	\includegraphics[width=0.8\textwidth]{Figures/pdfGeneralSDEusingGC.eps}
	\end{minipage}
	\caption{left: Probabilistic program representation of the SDE in Equation~\eqref{eq:SDE2} (left panel).  Histogram of sampled data from $x$ from executing the PP (sample size=1000, loop iteration=1000), the GC estimate of the underlying distribution in red  and the kernel density estimate of the sampled data in blue (right). The first 6 empirical moments are used for the GC  estimation. %Right: CDF (GC estimate and the sampled distribution).
	}
	\label{fig:HistogramPDFCDFofGeneralLoopEx1}
\end{figure}
% \begin{align}
% &x:=2\\\notag
% &w:=0\\\notag
% &dt:=1\\\notag
% &\sigma:=0.1\\\notag
% &\text{while true:}\\\notag
% &\quad w:=\text{Normal}(0,1)\\\notag
% &\quad x:=x-\frac{1}{4}x^3\ast dt -\frac{1}{2}x^2\ast \sigma\ast w
% \end{align}

Currently,  we are not able to compute the true moments of this probabilistic program's variables. We can, nevertheless, approximate them by carrying out a Monte-Carlo experiment by running the program   and stopping at a fix loop iteration, in order to obtain empirical moments from sampled data. For  the specific value  of  $\sigma=0.1$,
% \Ahmad{parameter $\sigma=0.1$} \efi{which parameters?}, 
the program generates data whose histogram in the right panel of Fig.~\ref{fig:HistogramPDFCDFofGeneralLoopEx1} indicates the distribution for the output random variable $x$ is bimodal. Here we use the first 6 (empirical) moments  and apply the Gram-Charlier expansion  to reconstruct the target distribution. The GC estimated pdf and a kernel density estimate of the sampled data are plotted in Fig.~\ref{fig:HistogramPDFCDFofGeneralLoopEx1} (right). 
%%%%%%%%%%%%%%%%%%%%%%%%%%%%%%%%%%%%%%%%%%%%%%%%%%%%%%%%%%%%%%%%%%%%%%%%%

\newpage
Table~\ref{table:AbsoluteandRelativeErrors} shows our results on the \textit{Precision of Higher Moments}  (cf. Algorithm~\ref{fig:algo} and Section~\ref{ssec:methods-of-evaluation}) for presented benchmarks in Section~\ref{section:ImplEvaluation}.

\begin{table}[tpbh!]
    \centering
    \scalebox{0.7}{
 \begin{tabular}{c|c|c|l|l|l|l}
\hline
  {\bf Program}  &\#Mom. & Moment &   Exact Value$^{1}$  &Absol. sample error$^{2}$   & Absol. ME est. error$^{3}$ & Absol. GC est. error$^{3}$  \\
    & for est.& & & (relative error$^\ast$)&  (relative error$^\ast$) &  (relative error$^\ast$)\\
                         \hline
                         \hline

 \multirow{3}{*}{StutteringP}&&1& 210 & $5.69\times 10^{-2} (0.027\%)$  &$8.08\times 10^{-5} (0.00003\%)$&$4.71\times 10^{-5} (0.00002\%)$\\%\cline{2-6}
    &2&2& $4.4405 \times 10^4 $ &  $2.39 \times 10^{1} (0.053\%)$& $1.75 \times 10^{-2} (0.00003\%)$&$1.75 \times 10^{-2} (0.00003\%)$\\%\cline{2-6}
    &&3& $9.4536\times 10^6$  & $6.78 \times 10^{3} (0.0.072\%)$ & $9.21 \times 10^{1} (0.000974\%)$ & $9.25 \times 10^{1} (0.000978\%)$\\%\cline{2-6}
    &&4& $2.0260\times 10^9$  & $1.48 \times 10^{6} (0.073\%)$& $7.38 \times 10^{4} (0.00364\%)$   & $7.42 \times 10^{4} (0.00366\%)$\\%\cline{2-6}
    &&5& $4.3705\times 10^{11}$  & $2.17 \times 10^{8} (0.050\%)$ & $3.82 \times 10^{7} (0.00873\%)$ & $3.83 \times 10^{7} (0.00876\%)$ \\%\cline{2-6}
    &&6&  $9.4884\times 10^{13}$ & $5.51 \times 10^{9} (0.0058\%)$ & $1.60 \times 10^{10} (0.0168\%)$  & $1.60 \times 10^{10} (0.0168\%)$\\%\cline{2-6}
    &&7& $2.0729\times 10^{16}$  & $2.10 \times 10^{13} (0.101\%)$& $5.88 \times 10^{12} (0.0284\%)$  & $5.90 \times 10^{12} (0.0285\%)$\\%\cline{2-6}
    &&8& $4.5570\times 10^{18}$  &$1.12 \times 10^{16} (0.245\%)$ &  $1.99 \times 10^{15} (0.0438\%)$  & $2.00 \times 10^{15} (0.0439\%)$
    \\\hline
        \hline

 \multirow{3}{*}{Square$^{\ast\ast}$}&&1& 10100 & $1.66\times 10^1 (0.16\%)$  &  $1.11\times 10^{0} (0.011\%)$  & $7.97\times 10^{-3} (0.00007\%)$ \\%\cline{2-6}
    &2&2& $1.0602 \times 10^8$ & $2.31\times 10^5 (0.22\%)$ & $2.30\times 10^3 (0.00217\%)$   & $1.64\times 10^{2} (0.00015\%)$ \\%\cline{2-6}
    &&3& $1.1544\times 10^{12}$  &$1.27\times 10^{9} (0.11\%)$  &  $1.26\times 10^7 (0.0011\%)$  &$2.39\times 10^{9} (0.2072\%)$\\%\cline{2-6}
    &&4& $1.3012\times 10^{16}$  & $2.98\times 10^{13} (0.23\%)$& $1.99\times 10^{12} (0.0153\%)$   &$9.79\times 10^{13} (0.7581\%)$ \\%\cline{2-6}
    &&5& $1.5157\times 10^{20}$  & $1.32\times 10^{18} (0.87\%)$& $8.83\times 10^{16} (0.0583\%)$    &$2.61\times 10^{18} (1.7505\%)$
    \\\hline
        \hline

\multirow{3}{*}{Binomial}&&1& 50 & $2.95\times 10^{-1} (0.59\%)$  &  $5.19\times 10^{-5} (0.000051\%)$ & $3.16\times 10^{-3} (0.0063\%)$\\%\cline{2-6}
    &2&2&   2525  & $2.82\times 10^{1} (1.12\%)$ & $2.74\times 10^{-3} (0.000108\%)$  & $1.87\times 10^{-1} (0.0074\%)$ \\%\cline{2-6}
    &&3& 128750  & $2.04\times 10^{3} (1.59\%)$ & $1.43\times 10^{-1} (0.000111\%)$  & $1.22\times 10^{1} (0.0095\%)$ \\%\cline{2-6}
    &&4&  $6.6268\times 10^{6}$  &$1.32\times 10^{5} (2.00\%)$ & $3.66\times 10^{0} (0.000055\%)$  & $8.22\times 10^{2} (0.0125\%)$ \\%\cline{2-6}
    &&5&  $3.4421\times 10^{8}$ &$8.08\times 10^{6} (2.35\%)$ &  $5.52\times 10^{2} (0.000160\%)$ & $5.53\times 10^{4} (0.0161\%)$ \\%\cline{2-6}
    &&6& $1.8038\times 10^{10}$ & $4.67\times 10^{8} (2.64\%)$& $1.20\times 10^{5} (0.000664\%)$   & $3.66\times 10^{6} (0.0203\%)$\\%\cline{2-6}
    &&7&  $9.5354\times 10^{11}$ &$2.74\times 10^{10} (2.87\%)$ &  $1.51\times 10^{7} (0.001587\%)$  & $2.38\times 10^{8} (0.0250\%)$\\%\cline{2-6}
    &&8&  $5.0830\times 10^{13}$ &$1.54\times 10^{12} (3.04\%)$ &  $1.54\times 10^{9} (0.0030363\%)$   & $1.51\times 10^{10} (0.0298\%)$
         \\\hline
        \hline

 \multirow{3}{*}{RandomWalk1D}&&1& 20 & $1.57\times 10^{-1} (0.79\%)$  &$1.83\times 10^{-6} (0.000009\%)$ & $4.44\times 10^{-3} (0.022\%)$\\%\cline{2-6}
    &2&2& $4.2933\times 10^{2} $ &  $6.78 \times 10^{0} (1.58\%)$& $6.76 \times 10^{-5} (0.00001\%)$ & $1.90\times 10^{-1} (0.0044\%)$\\%\cline{2-6}
    &&3& $9.7516\times 10^{3}$  & $2.45 \times 10^{2} (2.51\%) $& $8.40 \times 10^{0} (0.09\%)$  & $5.61\times 10^{-1} (0.0057\%)$\\%\cline{2-6}
    &&4&  $2.3230\times 10^{5}$ & $8.38\times 10^{3} (3.61\%)$&  $6.48\times 10^{2} (0.28\%)$  & $3.54\times 10^{2} (0.15\%)$\\%\cline{2-6}
    &&5& $5.7681\times 10^{6}$  & $2.79\times 10^{5} (4.48\%)$&  $3.37\times 10^{4} (0.58\%)$ &$2.32\times 10^{4} (0.40\%)$ \\%\cline{2-6}
    &&6&  $1.4858\times 10^{8}$ & $9.19\times 10^{6} (6.19\%)$&  $1.48\times 10^{6} (0.98\%)$ & $1.12\times 10^{6} (0.75\%)$ \\%\cline{2-6}
    &&7& $3.9565\times 10^{9}$  & $3.03\times 10^{8} (7.66\%)$& $5.94\times 10^{7} (1.48\%)$  & $4.72\times 10^{7} (1.18\%)$ \\%\cline{2-6}
    &&8& $1.0857\times 10^{11}$  & $1.01\times 10^{10} (9.26\%)$&  $2.26\times 10^{9} (2.04\%)$  & $1.85\times 10^{9} (1.67\%)$
    \\\hline
        \hline

 \multirow{3}{*}{Uniform (Cont.)}&&1& 0.5 & $5.92\times 10^{-3} (1.18\%)$  & $1.47\times 10^{-9} (3\times 10^{-7}\%)$ & $3.28\times 10^{-2} (7.03\%)$\\%\cline{2-6}
    &6&2& 0.333333 & $4.94\times 10^{-3} (1.48\%)$ &   $1.66\times 10^{-5} (0.00499\%)$& $3.40\times 10^{-2} (11.36\%)$\\%\cline{2-6}
    &&3& 0.25  & $4.57\times 10^{-3} (1.83\%)$ & $2.50\times 10^{-5} (0.00998\%)$  & $3.46\times 10^{-2} (16.06\%)$ \\%\cline{2-6}
    &&4&  0.20  &$4.57\times 10^{-3} (2.28\%)$ &  $3.33\times 10^{-5} (0.0166\%)$  & $3.43\times 10^{-2} (20.69\%)$\\%\cline{2-6}
    &&5&  0.166667  & $4.66\times 10^{-3} (2.80\%)$&   $4.18\times 10^{-5} (0.0249\%)$ &$3.35\times 10^{-2} (25.18\%)$ \\%\cline{2-6}
    &&6&  0.142857 &$4.74\times 10^{-3} (3.32\%)$ &   $4.99\times 10^{-5} (0.0349\%)$ & $3.25\times 10^{-2} (29.51\%)$\\%\cline{2-6}
    &&7&  0.125 &$4.76\times 10^{-3} (3.81\%)$ &     $5.82\times 10^{-5} (0.00465\%)$ &$3.15\times 10^{-2} (33.65\%)$\\%\cline{2-6}
    &&8&  0.1111111 &$4.73\times 10^{-3} (4.25\%)$ &  $6.66\times 10^{-5} (0.00599\%)$ &  $3.04\times 10^{-2} (37.60\%)$
         
    \\\hline
        \hline

 \multirow{3}{*}{PDP Model$^{\ast\ast}$}&&1& $1.1885\times 10^{3}$ & $1.60\times 10^{1}  (1.35\%)$  &$2.84\times 10^{-1}  (0.024\%)$ &$5.74\times 10^{0}  (0.48\%)$ \\%\cline{2-6}
    &3&2& $1.4767\times 10^{6}$ &  $3.93\times 10^{4} (2.66\%)$& $3.95\times 10^{2} (0.027\%)$ &$1.16\times 10^{4} (0.78\%)$ \\%\cline{2-6}
    &&3& $1.8981\times 10^{9}$  & $7.37 \times 10^{7} (3.88\%)$& $3.19\times 10^{6}(0.168\%)$ & $2.35\times 10^{7} (1.23\%)$\\%\cline{2-6}
     &&4& $2.5058\times 10^{12}$ & $1.28\times 10^{11}(5.01\%)$ &  $1.64\times 10^{10}$ (0.650\%)  & $4.85\times 10^{10} (1.90\%)$\\%\cline{2-6}
     &&5& $3.3804\times 10^{15}$  &$2.04\times 10^{14}(6.03\%)$  & $ 4.97\times 10^{13}$ (1.450\%) & $1.00\times 10^{14} (2.87\%)$\\%\cline{2-6}
%      &&6& $9.31994079132823\times 10^{17}$  & $6.33\times 10^{16}(6.79\%)$& $2.16\times 10^{16}$ (2.27\%)   & $6.42\times 10^{15} (0.6842\%)$ \\%\cline{2-6}
%      &&7& $1.04195827518657\times 10^{21}$  & $9.27\times 10^{19}(8.90\%)$&  $4.11\times 10^{19}$ (3.79\%)  & $1.46\times 10^{19} (1.3837\%)$ \\%\cline{2-6}
%      &&8& $1.19415322490998\times 10^{24}$
%   & $1.33\times 10^{23}(11.18\%)$& $7.23\times 10^{22}$ (5.71\%)   
%     & $2.95\times 10^{22} (2.4119\%)$\\\hline
        \hline

\end{tabular}
}
\vspace{2mm} 
 \caption{Error for Benchmarks:\\
 $^{1}$ Exact value of moments at the iteration loop $n=100$ (See Appendix~\ref{Appendix}: Table ~\ref{Table:Benchmarks})\\
 $^{2}$ Error of exact moments and sample moments\\
 $^{3}$ Error of exact moments and the ones calculated by the  estimated distribution\\
 $^\ast$ Relative error ($\%$)=$\frac{\text{Absolute Error}}{\text{Exact Value}}\times 100$\\
 $^{\ast\ast}$Moments of order above 5  could not be computed within ~30 minutes
 }
%  \label{Table:ErrorforBenchmarks}
\label{table:AbsoluteandRelativeErrors}
\end{table}

\newpage
